# Supplementary material for: SuRF: a New Method for Sparse Variable Selection, with Application in Microbiome Data Analysis
Source: arXiv:1909.06439 source file (2019-09-13)
Supplement: Supplementary file 1 [file SuRF_Supplemental.pdf]

# Web-based Supplementary Materials for "SuRF: a New Method for Sparse Variable Selection, with Application in Microbiome Data Analysis" by Lihui Liu, Hong Gu, Johan Van Limbergen and Toby Kenney

# Appendix A: Algorithm for variable selection procedures

**Algorithm 1** Variable ranking

**Require:** $X$ matrix of predictors (e.g. proportions for OTU data)

**function** VRANK($X_{N \times P}, y_N, q, B$)
  Step1: Create a zero matrix $M_{BP}$
  **for** $i \leftarrow 1$ to $B$ **do**
    Randomly select the $i^{th}$ stratified subsample of size qN;
    Fit lasso with this subsample;
    $M[i, T_i] = 1$; ▷ $T_i$ selected variable set chosen from $i^{th}$ subsampling
  **end for**
  Step2: Rank variables by their frequencies $F_q = \sum_b M[b, q]$;
  Step3: In case of a tie, re-rank variables according to the contribution of how each of them decreases the LR statistics by adding each variable to a model already including the variables listed above those tied variables;
  Step4: Further reduce the above list by removing the variables listed at the bottom with a low frequency.
  **return** $R = \{R_1, R_2, \ldots, R_{P'}\}$
▷ $R$ represents the ranked variable set (from most frequently selected to the least frequently selected)
**end function**

**Algorithm 2** Variable selection (main)

**function** VSELECT($X_{N\times P}, y_N, R, T$) ▷ $T$: the number of permutations

$C \leftarrow R$ ▷ $C$: Candidate variable set

$S \leftarrow \emptyset$ ▷ $S$: Selected variable set

**repeat**

newcutoff=DeriveSampDist($X_{N\times P}, y_N, C, S, T$);

$x^\star$=SelnNewvar($X_{N\times P}, y_N, C, S$, newcutoff)

$S \leftarrow \{S, x^\star\}$

$C \leftarrow \{C \backslash x^\star\}$

**until**

All observations have been perfectly classified or $x^\star == \emptyset$

**return**

**end function**

**Algorithm 3** Variable selection step 1: derive the sampling distribution

**function** DERIVESAMPDIST($X_{N \times P}, y_N, C, S, T, \alpha = 0.05$) ▷ $T$: the number of permutations
    **for** $i \leftarrow 1$ to $T$ **do**
        Select a random permutation $\pi_i$
        Permute all rows of variables listed in $C$ with $\pi_i$

        **for** $j \leftarrow 1$ to $w$ **do** ▷ $w = |C|$: the size of the set
            $P_j \leftarrow \{S, C_j\}$
            $D_j \leftarrow -2 \ln \frac{L_S}{L_{P_j}}$
        **end for**
        $D_i^{max} \leftarrow \max_j D_j$
    **end for**
    $D_{1-\alpha}^{max} \leftarrow \{D_1^{max}, \ldots, D_T^{max}\}_{1-\alpha}$ ▷ $D_{1-\alpha}^{max}$: the new cut-off value
    **return** $D_{1-\alpha}^{max}$

**end function**

$D_j$ Likelihood ratio statistics between model using variables in $S$ and in $L_{P_j}$

$L_S$: Likelihood of the model including variables in the current selected variable set S

$L_{P_j}$: Likelihood of the model including variables in the current selected variable set S plus the $j^{th}$ candidate variable in candidate set C

**Algorithm 4** Variable selection step 2: select a new variable

**function** SelNewVar($X_{N\times P}, y_N, C, S, newC$)
  **for** $k \leftarrow 1$ to $w$ **do** ▷ $w = |C|$: the size of the set
    $P_k \leftarrow \{S, C_k\}$
    $G_k \leftarrow -2 \ln \frac{L_S}{L_{P_k}}$
    **if** $G_k > newC$ **then**
      **return** $xnew = C_k$;break;
    **end if**
  **end for**
  **return** $\emptyset$
  $G_k$ Likelihood ratio statistics between model using variables in $S$ and in $L_{P_k}$
  $L_S$: Likelihood of the model including variables in the current selected variable set S
  $L_{P_k}$: Likelihood of the model including variables in the current selected variable set S plus the $k^{th}$ candidate variable in candidate set C
**end function**

# Appendix B: Proofs of Theorems

**Theorem 1.** *Suppose we have a true model $\mathbb{E}(Y|X) = g^{-1}(X\beta)$, where $Y|X$ follows an exponential family distribution, $g$ is a link function, and $\beta_i$ is zero for all but a fixed number $p_{true}$ of predictors. Suppose further that we have already selected the set $S$ of variables, all of which satisfy $\beta_j \neq 0$ and that there is at least one variable $i \notin S$ with $\beta_i \neq 0$. Let $D(k)$ be the log-likelihood ratio statistic for the variable $k$. Then there is some $j \notin S$ with $\beta_j \neq 0$ such that $D(j) = O(n)$.*

*Proof.* For this proof, we will need to introduce some notation. Let $\beta^*_S$ be the optimal coefficients for the model under the restriction $\beta_i = 0$ for all $i \notin S$ (where optimality means minimising the expectation over $X$ of the Kullback-Leibler divergence between the fitted conditional distribution and the true conditional distribution). We let $\widehat{\beta_S}$ be the coefficients estimated from the data. We have that

$$\begin{aligned} D(k) &= l(X, \widehat{\beta_{S\cup\{k\}}}) - l(X, \widehat{\beta_S}) \\ &= l(X, \beta^*_{S\cup\{k\}}) - l(X, \beta^*_S) + \left(l(X, \widehat{\beta_{S\cup\{k\}}}) - l(X, \beta^*_{S\cup\{k\}})\right) - \left(l(X, \widehat{\beta_S}) - l(X, \beta^*_S)\right) \end{aligned}$$

From standard likelihood theory, the statistics $l(X, \widehat{\beta_{S\cup\{k\}}}) - l(X, \beta_{S\cup\{k\}})$ and $l(X, \widehat{\beta_S}) - l(X, \beta_S)$ are asymptotically stochastically dominated by distributions which do not depend on $n$. (In particular, for any fixed set of variables $S$, the difference $l(X, \widehat{\beta_S}) - l(X, \beta^*_S)$ follows a chi-square distributions with $|S|$ degrees of freedom. Therefore, if $S$ is chosen from all the subsets of true predictors of a given size, then $l(X, \widehat{\beta_S}) - l(X, \beta^*_S)$ is bounded by the maximum over all $\binom{p_{\text{true}}}{|S|}$ such chi-square distributions. If $S(x)$ is the survival function for each chi-square distribution, the survival function for the maximum is bounded by $\binom{p_{\text{true}}}{|S|}S(x)$, which does not depend on $n$.)

Meanwhile $\frac{l(X,\beta^*_{S\cup\{k\}}) - l(X,\beta^*_S)}{n}$ tends to $\mathbb{E}_X(l(X, \beta^*_{S\cup\{k\}})) - \mathbb{E}_X(l(X, \beta^*_S))$, so provided we have that $\mathbb{E}_X(l(X, \beta^*_{S\cup\{k\}})) > \mathbb{E}_X(l(X, \beta^*_S))$, we will have that $D(k) = O(n)$. We just need to show that for some $k$, this expression holds. Let $\beta$ be the vector which maximises $\mathbb{E}(l(X, \beta))$ and let $T$ be the set of coefficients of $\beta$ which are non-zero. We have assumed that $S \subsetneqq T$. We know that for an exponential family model, the likelihood function is concave. This means that if $\beta^*_S$ is not the global maximum for $\mathbb{E}(l(X, \beta))$, then it

must have a non-zero derivative in the direction $\beta - \beta_S^*$. Since it has a non-zero derivative, in this direction, it must have non-zero derivative in one of the component directions. Let $k$ be one of the component directions in which there is a non-zero derivative. Then we must have $\mathbb{E}(l(X, \beta^*_{S\cup\{k\}})) > \mathbb{E}(l(X, \beta^*_S))$, which completes the proof. □

On the other hand, we can study how the null distribution changes with $n$ and $p$.

**Theorem 2.** *Suppose $X$ is an $n \times p$ matrix and $Y$ is a random vector (independent of $X$) from the exponential family distribution fitted by the model , then the maximum deviance of a single column of $X$ as a predictor of $Y$ has survival function bounded by $S(x) \leqslant \frac{2pe^{-\frac{x}{2}}}{\sqrt{2\pi x}}$.*

*Proof.* For a single column of $X$, the deviance asymptotically follows a chi-square distribution with one degree of freedom. Its survival function is therefore $S(x) = 2\Phi(-\sqrt{x})$. The survival function of the maximum of $p$ such distributions is therefore bounded by $S(x) \leqslant 2p\Phi(-\sqrt{x})$ (with no assumptions about the joint distribution). Recall for $u < 0$, we have

$$\begin{aligned}
\Phi(u) &= \int_{-\infty}^{u} \frac{e^{-\frac{t^2}{2}}}{\sqrt{2\pi}}\,dt \\
&\leqslant \int_{-\infty}^{u} \frac{t}{u}\frac{e^{-\frac{t^2}{2}}}{\sqrt{2\pi}}\,dt \\
&= \frac{1}{\sqrt{2\pi}u}\left[-e^{-\frac{t^2}{2}}\right]_{-\infty}^{u} \\
&= \frac{-e^{-\frac{u^2}{2}}}{\sqrt{2\pi}u}
\end{aligned}$$

In particular, setting $u = -\sqrt{x}$ gives us $S(x) \leqslant 2p\Phi(-\sqrt{x}) \leqslant 2p\frac{e^{-\frac{x}{2}}}{\sqrt{2\pi x}}$ This means that the survival function is bounded by $\frac{2pe^{-\frac{x}{2}}}{\sqrt{2\pi x}}$. □

# Appendix C: Simulation Study 3

## Design

This simulation provides a larger scale simulation to determine the performance of SuRF under different conditions. We base this simulation on the

OTU counts from the Left Palm data of the moving picture data set. This data set includes over 12,000 OTUs, many more than in the previous simulations. Furthermore, in this simulation, we include 8 true variables, to assess the performance of SuRF in less sparse situations. We choose the true predictors to assess the influence of various factors on the ability of SuRF to select key predictors. In particular, we choose 8 predictors across a range of taxonomic levels, with some rarer taxa, and several different nesting patterns between the taxa. The nesting patterns and rareness are shown in Web Figure 1. We choose a chain of abundant variables from the class Bacilli; the phylum Bacteroidetes and two classes within it; the phylum Synergistetes; and the species *Corynebacterium tuberculostearicum.* All the variables used have at least one strong surrogate in the dataset (correlation at least 0.9), with the exception of A2 and B.

We also study the effect of the coefficients on the taxa selected, simulating two different sets of coefficients, one with larger coefficients for abundant taxa, and one with larger coefficients for rare taxa. For each set of coefficients, we simulated a high, medium and low signal-noise ratio. For each simulation, we simulated 100 datasets. Web Table 1 gives the coefficients for these simulations.

## Results

Web Table 8 summarises the results of SuRF, Stability selection and LASSO on these simulations.

This is a very challenging problem with slightly over 300 observations and over 12,000 variables. This explains why the results are generally worse than Simulation 2. We see that SuRF significantly outperforms the other methods in all scenarios in terms of misclassification error rate, and in terms of number of noise variables selected. SuRF does not achieve the target 0.05 noise variables, but selects sparse models. SuRF also selects more true variables than Stability in all scenarios, and more than LASSO in many situations. LASSO selects a lot of variables, so would be expected to select more true variables by chance. As expected, the number of true variables selected increases as signal-noise ratio increases. With even higher SNR, or more data, we would expect SuRF to select all the true variables.

We now look at patterns among which true variables are selected. Web Table 9 shows the number of times each of the true variables was selected by each method in each scenario.

In the first scenario (S1), we see that as expected, variables with larger coefficients are selected more often. Even at high signal-noise ratio, Sphingobacteria was never selected, and *Thermoactinomycetaceae* was rarely selected. However, we also see that among variables with the same coefficients, *Corynebacterium tuberculostearicum* was selected a reasonable proportion of times, while Synergistetes and Bacteroidetes were never selected. This indicates that it may be easier to select abundant predictors. In the case of Bacteroidetes, the effect is absorbed by the class Bacteroidia. In the class Bacilli, the class-level variable is often selected instead of the order Bacillales. The high correlation between the order-level and class-level variables makes distinguishing between them a challenging problem, and among the three methods, only SuRF is able to detect that both have a separate effect, when the signal noise ratio is high.

LASSO also shows similar patterns of favouring more abundant variables from among variables with the same coefficients. Stability selection mostly selected only Bacteroidia, so it is not possible to determine the extent to which it might favour more abundant taxa from the results on this scenario.

In Scenario 2, we see that even when coefficients are larger for rare taxa, the methods still have difficulty selecting these variables. This is an issue with penalised logistic regression, where the underlying distribution of the predictor variable can have a large effect on that variable's ability to be selected. We plan to address this issue in future research. This issue is even more significant for LASSO, which never selects Synergistetes, in spite of the large coefficient. Stability selection also shows some ability to select the abundant predictors Bacteroidetes and Bacteroidia, but cannot select the rare predictors Sphingobacteria or Synergistetes. It is able to select the rare predictor *Corynebacterium tuberculostearicum.* This is presumably related to the problem of selecting between correlated variables. When there are closely correlated variables, stability selection will often select neither, while SuRF will usually select one, and can select both if there is evidence for separate effects from the two variables.

It is also interesting to look at the selection between surrogates. Many of the true variables in the simulation have strong surrogates in the data. Looking more carefully, we see that for this data set, SuRF is often able to distinguish between surrogates with correlation less than 0.95, whereas the other methods, when they select any variables, tend to have more difficulty determining which surrogate variable should be selected.

# Appendix D: $p$-values

In this section, we study the reliability of the $p$-values given by SuRF. The $p$-value calculated by SuRF represents the $p$-value for the null hypothesis that all true predictors have already been included in the model. Because of the presence of surrogate variables, if there are true predictors that have not been included in the model, this null hypothesis may be rejected even if the next variable selected is not the "true predictor". Therefore, we can only assess the reliability of this $p$-value in the simulations by examining cases where all true variables have already been selected. Recall that SuRF is a forward selection method, so there is an order in which variables enter the model. If a noise variable enters the model before all true variables have been selected, then it is technically correct to reject the null hypothesis that all true variables have been selected.

If the probability of rejecting the null hypothesis is $p$, then the number of variables selected after all true variables have already been selected should follow a geometric distribution with parameter $1 - p$. The total number of noise variables selected across all simulations therefore should follow a negative binomial distribution with $r$ the number of simulations in which all true variables are selected, and $p$ the probability of incorrectly rejecting the null hypothesis. Thus if $N$ is the number of cases in which we select all true predictors and $X$ is the number of noise variables selected after all true variables, then the MLE estimate for $p$ is $\frac{X}{X+N}$. If our $p$-values are well controlled, then we should have $p = 0.05$. We can test the significance of the number of noise variables selected with the null hypothesis $p = 0.05$ and the alternative hypothesis $p > 0.05$. The significance is given by

$$\sum_{x=X}^{\infty} \binom{x+N}{N} 0.05^x 0.95^N$$

We calculate the number of cases where all true variables are selected, and the number of noise variables that are selected after all true variables for Simulations 1 and 2 in Web Table 12. We cannot assess reliability for Simulation 3 because there were no cases where all true predictors were selected.

We see that the results are consistent with the $p$-values being correct. Only in one case, (Simulation 1, Scenario 2, fair SNR) is the number of noise variables selected after all true variables significantly more than would be

expected for a reliable $p$-value. When accounting for the multiple testing from the 18 different scenarios, this is not significant.

# Web Tables

**Web Table 1:** Coefficients used in the simulations. Each coefficient is the product of the relative variable coefficient shown at the top for each scenario, and the factor for signal-noise ratio.

| | SNR | factor | variable coefficient | | | | | | | |
|---|---|---|---|---|---|---|---|---|---|---|
| | | | A | A1 | A2 | B | B1 | B2 | C | D |
| | | | 1 | 1.5 | −0.5 | 1 | 2 | −0.5 | 1 | 1 |
| S1 | High | 1.72 | 1.72 | 2.58 | −0.86 | 1.72 | 3.44 | −0.86 | 1.72 | 1.72 |
| | Fair | 0.75 | 0.75 | 1.125 | −0.375 | 0.75 | 1.5 | −0.375 | 0.75 | 0.75 |
| | Low | 0.63 | 0.63 | 0.945 | −0.315 | 0.63 | 1.26 | −0.315 | 0.63 | 0.63 |
| | | | 1 | 1 | 2 | 1 | 1 | 2 | 2 | 1 |
| S2 | High | 1.9 | 1.9 | 3.8 | 1.9 | 1.9 | 3.8 | 3.8 | 1.9 | 1.9 |
| | Fair | 0.794 | 0.794 | 1.588 | 0.794 | 0.794 | 1.588 | 1.588 | 0.794 | 0.794 |
| | Low | 0.613 | 0.613 | 1.226 | 0.613 | 0.613 | 1.226 | 1.226 | 0.613 | 0.613 |

**Web Table 2:** List of top 10 variables for Pouch by SuRF

| **Variable Name** | **Taxonomy Level** | **Phylum** | **Frequency** | **LR Statistics** | ***p*-value** | **Critical Value** |
|---|---|---|---|---|---|---|
| **Bacteroidetes** | Phylum | Bacteroidetes | 923 | **32.45** | 0.000 | **13.36** |
| **Fusobacteriaceae** | Family | Fusobacteria | 232 | 5.96 | 0.995 | 13.76 |
| **unclassified** | Order | Proteobacteria | 225 | 2.46 | 1.000 | |
| **Turicibacter** | Genus | Firmicutes | 220 | 6.53 | 0.965 | |
| **Subdoligranulum** | Genus | Firmicutes | 179 | 5.61 | 0.995 | |
| **Bacteroidia** | Class | Bacteroidetes | 170 | 0.03 | 1.000 | |
| **Erysipelotrichi** | Class | Firmicutes | 151 | 3.92 | 1.000 | |
| **Bacilli** | Class | Firmicutes | 150 | 2.85 | 1.000 | |
| **Dialister** | Genus | Firmicutes | 141 | 11.03 | 0.315 | |
| **Granulicatella** | Genus | Firmicutes | 131 | 2.90 | 1.000 | |

**Web Table 3:** List of top 10 variables for Afferent Limb by SuRF

| **Variable Name** | **Taxonomy Level** | **Phylum** | **Frequency** | **LR Statistics** | ***p*-value** | **Critical Value** |
|---|---|---|---|---|---|---|
| **Bacteroidetes** | Phylum | Bacteroidetes | 858 | **24.53** | 0.000 | **12.75** |
| **Bacteroidia** | Class | Bacteroidetes | 322 | 0.03 | 1.000 | 14.29 |
| **Erysipelotrichi** | Class | Firmicutes | 188 | 5.21 | 1.000 | |
| **Pasteurellales** | Order | Proteobacteria | 163 | 9.60 | 0.415 | |
| **Bacilli** | Class | Firmicutes | 149 | 11.18 | 0.180 | |
| **unclassfied** | Genus | Firmicutes | 144 | 10.80 | 0.230 | |
| **Epsilonproteobacteria** | Class | Proteobacteria | 139 | 6.05 | 0.980 | |
| **Deinococcus-Thermus** | Phylum | Deinococcus-Thermus | 138 | 4.51 | 1.000 | |
| **Leuconostocaceae** | Family | Firmicutes | 138 | 5.56 | 0.995 | |
| **unclassfied** | Genus | Bacteroidetes | 134 | 5.62 | 0.995 | |

**Web Table 4:** Summary of selected variables for 4 body sites by SuRF

| Site | Selected variable | Last known level | Phylum | Critical value | LR | $p$-value |
|---|---|---|---|---|---|---|
| Gut | unclassified species | *Bacteroides Genus* | Bacteroidetes | 17.77 | 371.21 | 0.00 |
| Tongue | unclassified species | Lachnospiraceae Family | Firmicutes | 14.90 | 309.45 | 0.00 |
| | unclassified species | *Neisseria Genus* | Proteobacteria | 18.13 | 43.18 | 0.00 |
| | unclassified species | Sphingobacteriales Order | Firmicutes | 26.12 | 28.67 | 0.01 |
| Left Palm | unclassified species | *Deinococcus Genus* | Thermi | 20.29 | 327.79 | 0.00 |
| | *Propionibacterium Genus* | *Propionibacterium Genus* | Actinobacteria | 17.28 | 56.97 | 0.00 |
| Right Palm | unclassified species | *Corynebacterium Genus* | Actinobacteria | 20.82 | 169.26 | 0.00 |
| | unclassified species | *Deinococcus Genus* | Thermi | 19.85 | 187.77 | 0.00 |

**Web Table 5:** Simulation study 1 complete results

| Senario | | **SuRF** | **Stability** 0.6 | 0.7 | 0.8 | 0.9 | **VSURF** | **LASSO** |
|---|---|---|---|---|---|---|---|---|
| | | | | (a) **Null Case** [1] | | | | |
| | | 5 | 200 | 200 | 200 | 1 | 200 | 13 |
| *Null* | mean | 0.03 | 13.10 | 8.06 | 3.01 | 0.01 | 3.96 | 0.92) |
| | (SD) | (0.18) | (0.67) | (0.56) | (0.27) | (0.07) | (2.64) | (5.15) |
| | SNR | | | (b) **True positive results** over 100 simulations [2] | | | | |
| S1 | High | 100 | 98 | 92 | 80 | 58 | 82 | 100 |
| | Fair | 98 | 88 | 69 | 48 | 26 | 79 | 100 |
| | Low | 95 | 81 | 65 | 39 | 16 | 83 | 95 |
| S2 | High | 100 | 100 | 100 | 100 | 100 | 100 | 100 |
| | Fair | 100 | 100 | 100 | 100 | 93 | 93 | 95 |
| | Low | 97 | 99 | 96 | 91 | 71 | 83 | 87 |
| S3 | High | 100 (100) | 90 (100) | 80 (100) | 60 (100) | 24 (100) | 86 (100) | 100 (100) |
| | Fair | 66 (100) | 72 (99) | 40 (98) | 19 (90) | 3 (63) | 63 (94) | 88 (99) |
| | Low | 35 (96) | 43 (92) | 25 (84) | 9 (74) | 1 (46) | 49 (93) | 70 (98) |
| S4 | High | 19 (100) | 22 (100) | 10 (100) | 3 (100) | 1 (100) | 8 (100) | 57 (99) |
| | Fair | 9 (100) | 14 (100) | 11 (99) | 8 (92) | 2 (62) | 16 (98) | 84 (84) |
| | Low | 8 (92) | 8 (98) | 4 (94) | 0 (80) | 0 (32) | 5 (94) | 20 (66) |
| | | | | (c) **False positive results:** average number of noise variables (SD) over 100 simulations | | | | |
| S1 | High | **0.02** (0.14) | 4.06 (2.18) | 2.88 (1.94) | 1.66 (1.39) | 0.46 (0.63) | 4.50 (3.11) | 22.45(21.62) |
| | Fair | **0.11** (0.35) | 1.78 (1.51) | 1.17 (1.20) | 0.56 (0.88) | 0.15 (0.46) | 4.76 (3.13) | 31.46(43.69) |
| | Low | 0.09 (0.32) | 1.24 (1.20) | 0.76 (0.87) | 0.38 (0.60) | **0.04** (0.20) | 4.58 (3.30) | 42.96 (55.03) |
| S2 | High | 0.06 (0.24) | 0.56 (1.09) | 0.24 (0.71) | 0.06 (0.28) | **0.00** (0.00) | 5.77 (2.97) | 24.04 (25.64) |
| | Fair | 0.11 (0.31) | 0.89 (1.16) | 0.89 (1.16) | 0.89 (1.16) | **0.08** (0.34) | 5.26 (2.87) | 33.92 (37.04) |
| | Low | 0.07 (0.26) | 0.93 (1.37) | 0.61 (1.05) | 0.18 (0.48) | **0.02** (0.14) | 5.00 (2.82) | 29.52 (42.46) |
| S3 | High | 0.05 (0.22) | 0.54 (0.81) | 0.31 (0.66) | 0.06 (0.24) | **0.01** (0.10) | 2.49 (2.27) | 18.79 (32.51) |
| | Fair | 0.06 (0.24) | 0.81 (1.04) | 0.45 (0.77) | 0.24 (0.26) | **0.04** (0.20) | 4.15 (2.76) | 31.57 (43.18) |
| | Low | 0.16 (0.40) | 1.12 (1.23) | 1.23 (0.74) | 0.29 (0.62) | **0.04** (0.20) | 4.12 (2.98) | 27.61 (37.27) |
| S4 | High | 0.08 (0.31) | 0.84 (1.14) | 0.37 (0.80) | 0.11 (0.51) | **0.03** (0.22) | 5.60 (2.85) | 26.24 (24.94) |
| | Fair | **0.11** (0.31) | 1.04 (1.45) | 1.09 (1.11) | 0.33 (0.90) | 0.14 (1.51) | 4.30 (2.52) | 19.56 (29.58) |
| | Low | 0.09 (0.29) | 0.82 (1.26) | 0.41 (0.95) | 0.15 (0.64) | **0.02** (0.14) | 4.33 (2.49) | 19.21 (33.25) |
| | | | | (d) **In-sample mean misclassficaition error rate (SD)** over 100 simulations | | | | |
| S1 | High | **0.095** (0.011) | 0.103 (0.044) | 0.115 (0.076) | 0.152 (0.130) | 0.252 (0.194) | 0.108 (0.031) | 0.126 (0.062) |
| | Fair | **0.190** (0.019) | 0.219 (0.080) | 0.264 (0.130) | 0.339 (0.157) | 0.416 (0.141) | 0.240 (0.048) | 0.365 (0.142) |
| | Low | **0.240** (0.082) | 0.274 (0.101) | 0.311 (0.127) | 0.381 (0.139) | 0.454 (0.107) | 0.276 (0.027) | 0.418 (0.120) |
| S2 | High | 0.093 (0.010) | 0.095 (0.011) | 0.094 (0.010) | **0.092** (0.009) | **0.092** (0.008) | 0.122 (0.018) | 0.224 (0.058) |
| | Fair | 0.173 (0.016) | 0.178 (0.017) | 0.175 (0.016) | **0.172** (0.014) | 0.187 (0.074) | 0.222 (0.023) | 0.294 (0.104) |
| | Low | **0.210** (0.020) | **0.210** (0.020) | 0.214 (0.069) | 0.223 (0.088) | 0.282 (0.142) | 0.266 (0.024) | 0.368 (0.144) |
| S3 | High | **0.102** (0.010) | 0.115 (0.037) | 0.127 (0.048) | 0.151 (0.062) | 0.196 (0.056) | 0.124 (0.015) | 0.228 (0.063) |
| | Fair | 0.204 (0.080) | **0.192** (0.026) | 0.207 (0.029) | 0.231 (0.068) | 0.316 (0.133) | 0.232(0.021) | 0.311 (0.100) |
| | Low | 0.262 (0.129) | **0.232** (0.072) | 0.251 (0.097) | 0.282 (0.116) | 0.365(0.139) | 0.265 (0.026) | 0.342 (0.127) |
| S4 | High | **0.136** (0.030) | 0.139 (0.032) | 0.145 (0.031) | 0.147 (0.029) | 0.152 (0.045) | 0.117 (0.018) | 0.204 (0.059) |
| | Fair | **0.204** (0.016) | 0.207 (0.012) | 0.210 (0.032) | 0.231 (0.080) | 0.318 (0.147) | 0.220 (0.024) | 0.356 (0.160) |
| | Low | 0.245 (0.077) | **0.231** (0.055) | 0.242 (0.076) | 0.280 (0.114) | 0.408 (0.129) | 0.254 (0.025) | 0.403 (0.152) |

[1] Simulation under Null case: the number of batches that any noise variables are selected, together with mean and standard deviation of number of noise variables over 200 batches.

[2] In senario 1 and 2, the table gives the total number of times the true single variable/surrogate variable is selected. In senario 3, the table gives the total number of two true variables selected and the number of times at least one of two true variables selected in the bracket. In senario 4, the tables gives the number of times two true/surrogate variables selected (perfect selection) and the numer of times variables selected deemed correct selection in bracket.

**Web Table 6:** Simulation study 2 (Binary outcome) complete results

| SNR | No of true variables selected | SuRF | Stability 0.6 | Stability 0.7 | Stability 0.8 | Stability 0.9 | VSURF | LASSO | RF | SVM |
|---|---|---|---|---|---|---|---|---|---|---|
| **(a) Frequency of number of true varaibles selected over 100 simulations** | | | | | | | | | | |
| High | 3 | **99** | 0 | 0 | 0 | 0 | 20 | 30 | N/A | |
| | 2 | 1 | 4 | 12 | 13 | 14 | 80 | 70 | | |
| | 1 | 0 | 96 | 88 | 87 | 86 | 0 | 0 | | |
| | 0 | 0 | 0 | 0 | 0 | 0 | 0 | 0 | | |
| Fair | 3 | **82** | 0 | 0 | 0 | 0 | 21 | 5 | | |
| | 2 | 18 | 3 | 7 | 5 | 3 | 78 | 90 | | |
| | 1 | 0 | 97 | 93 | 95 | 97 | 1 | 5 | | |
| | 0 | 0 | 0 | 0 | 0 | 0 | 0 | 0 | | |
| Low | 3 | **71** | 0 | 0 | 0 | 0 | 9 | 4 | | |
| | 2 | 24 | 2 | 5 | 4 | 1 | 76 | 76 | | |
| | 1 | 5 | 97 | 95 | 96 | 97 | 15 | 20 | | |
| | 0 | 0 | 1 | 0 | 0 | 2 | 0 | 0 | | |
| **(b) Mean number of noise varaibles selected (sd)** | | | | | | | | | | |
| High | mean | **0.120** | 0.76 | 0.71 | 0.37 | **0.120** | 8.71 | 68.93 | N/A | |
| | SD | (0.356) | (0.452) | (0.556) | (0.544) | (0.327) | (3.036) | (40.59) | | |
| Fair | mean | 0.690 | 0.340 | 0.250 | 0.120 | **0.02** | 7.080 | 62.45 | | |
| | SD | (0.895) | (0.476) | (0.458) | (0.327) | (0.141) | (3.183) | (46.98) | | |
| Low | mean | 0.610 | 0.160 | 0.140 | 0.050 | **0.010** | 6.590 | 61.92 | | |
| | SD | (0.764) | (0.368) | (0.377) | (0.219) | (0.327) | (0.100) | (55.24) | | |
| **(c) Mean misclassfication error rate in test samples (sd)** | | | | | | | | | | |
| High | mean | **0.102** | 0.383 | 0.382 | 0.399 | 0.412 | 0.288 | 0.290 | 0.292 | 0.197 |
| | SD | (0.020) | (0.033) | (0.043) | (0.041) | (0.035) | (0.034) | (0.041) | (0.026) | (0.046) |
| Fair | mean | **0.191** | 0.366 | 0.369 | 0.373 | 0.377 | 0.301 | 0.323 | 0.291 | 0.372 |
| | SD | (0.028) | (0.034) | (0.033) | (0.033) | (0.030) | (0.041) | (0.038) | (0.032) | (0.080) |
| Low | mean | **0.228** | 0.361 | 0.359 | 0.361 | 0.366 | 0.315 | 0.333 | 0.296 | 0.390 |
| | SD | (0.038) | (0.037) | (0.032) | (0.031) | (0.035) | (0.047) | (0.033) | (0.032) | (0.084) |
| **(d) In-sample mean misclassfication error rate (sd)** | | | | | | | | | | |
| High | mean | **0.100** | 0.228 | 0.249 | 0.276 | 0.295 | 0.126 | 0.169 | 0.126 | 0.128 |
| | SD | (0.009) | (0.038) | (0.053) | (0.049) | (0.033) | (0.011) | (0.034) | (0.011) | (0.014) |
| Fair | mean | **0.220** | 0.309 | 0.324 | 0.340 | 0.350 | 0.259 | 0.295 | 0.259 | 0.277 |
| | SD | (0.010) | (0.030) | (0.031) | (0.024) | (0.010) | (0.017) | (0.029) | (0.017) | (0.024) |
| Low | mean | **0.259** | 0.348 | 0.357 | 0.364 | 0.371 | 0.285 | 0.331 | 0.285 | 0.317 |
| | SD | (0.017) | (0.031) | (0.029) | (0.022) | (0.012) | (0.020) | (0.034) | (0.020) | (0.032) |

**Web Table 7:** Simulation study 2 (Continuous outcome)

| SNR | No of true variables | SuRF | Stability 0.6 | Stability 0.7 | Stability 0.8 | Stability 0.9 | VSURF | LASSO | RF |
|---|---|---|---|---|---|---|---|---|---|
| | | | | **(a) Number of true variables selected** | | | | | |
| High | 3 | **99** | 0 | 0 | 0 | 0 | 81 | 35 | N/A |
| | 2 | 1 | 0 | 0 | 0 | 0 | 19 | 65 | |
| | 1 | 0 | 100 | 100 | 100 | 100 | 0 | 0 | |
| | 0 | 0 | 0 | 0 | 0 | 0 | 0 | 0 | |
| Fair | 3 | **97** | 0 | 0 | 0 | 0 | 71 | 12 | |
| | 2 | 3 | 0 | 0 | 0 | 2 | 19 | 81 | |
| | 1 | 0 | 100 | 100 | 100 | 98 | 0 | 7 | |
| | 0 | 0 | 0 | 0 | 0 | 0 | 0 | 0 | |
| Low | 3 | **80** | 0 | 0 | 0 | 0 | 40 | 1 | |
| | 2 | 19 | 4 | 4 | 4 | 2 | 60 | 52 | |
| | 1 | 1 | 96 | 96 | 96 | 98 | 0 | 47 | |
| | 0 | 0 | 0 | 0 | 0 | 0 | 0 | 0 | |
| | | | | **(b)Mean number of noise variables selected (sd)** | | | | | |
| High | mean | **0.040** | 0.360 | 0.260 | 0.160 | 0.080 | 15.16 | 52.540 | N/A |
| | SD | (0.197) | (0.503) | (0.463) | (0.368) | (0.273) | (4.334) | (29.186) | |
| Fair | mean | 0.140 | 0.790 | 0.680 | 0.370 | **0.100** | 4.436 | 46.370 | |
| | SD | (0.377) | (0.686) | (0.709) | (0.614) | (0.302) | (2.106) | (30.833) | |
| Low | mean | 0.540 | 0.700 | 0.290 | 0.110 | **0.010** | 14.330 | 28.700 | |
| | SD | (0.784) | (0.916) | (0.574) | (0.373) | (0.100) | (5.650) | (16.407) | |
| | Oracle MSE | | | **(c) Median MSE (IQR) in test samples** | | | | | |
| High | 1 | **1.009** | 4.433 | 4.380 | 4.475 | 4.555 | 2.781 | 3.470 | 2.977 |
| | | (0.131) | (0.672) | (0.758) | (0.774) | (0.678) | (0.379) | (0.794) | (0.416) |
| Fair | 1 | **1.004** | 2.870 | 2.917 | 3.069 | 3.117 | 2.083 | 2.535 | 2.236 |
| | | (0.143) | (0.430) | (0.454) | ( 0.496) | (0.357) | (0.258) | (0.460) | (0.272) |
| Low | 1 | **1.011** | 1.691 | 1.695 | 1.708 | 1.711 | 1.428 | 1.644 | 1.431 |
| | | (0.176) | (0.267) | (0.251) | (0.255) | (0.237) | (0.232) | (0.499) | (0.224) |
| | Average Oracle $R^2(sd)$ | | | **(d) Mean $R^2$ (sd) in test samples** | | | | | |
| High | 0.803 | **0.801** | 0.367 | 0.373 | 0.365 | 0.356 | 0.460 | 0.324 | 0.417 |
| | (0.018) | (0.010) | (0.044) | (0.058) | (0.057) | (0.046) | (0.048) | (0.109) | (0.038) |
| Fair | 0.749 | **0.706** | 0.389 | 0.381 | 0.357 | 0.336 | 0.391 | 0.267 | 0.359 |
| | (0.029) | (0.030) | (0.072) | (0.073) | (0.066) | (0.050) | (0.045) | (0.100) | (0.037) |
| Low | 0.455 | **0.439** | 0.274 | 0.262 | 0.257 | 0.253 | 0.215 | 0.127 | 0.211 |
| | (0.051) | (0.051) | (0.070) | (0.064) | (0.062) | (0.054) | (0.062) | (0.071) | (0.053) |
| | Oracle MSE | | | **(e) In-sample Median MSE (IQR)** | | | | | |
| High | 1 | **1.043** | 4.964 | 4.966 | 4.968 | 4.971 | 1.655 | 1.723 | 1.698 |
| | | (0.010) | (0.816) | (0.216) | (0.016) | (0.015) | (0.092) | (0.100) | (0.099) |
| Fair | 1 | **1.025** | 2.796 | 2.810 | 3.338 | 3.340 | 1.498 | 1.487 | 1.535 |
| | | (0.010 | (0.646) | (0.648) | (0.559) | (0.010) | (0.103) | (0.079) | (0.101) |
| Low | 1 | **1.071** | 1.993 | 1.997 | 1.999 | 2.000 | 1.555 | 1.312 | 1.570 |
| | | (0.018) | (0.155) | (0.013) | (0.011) | (0.011) | (0.089) | (0.035) | (0.100) |
| | Oracle $R^2$ | | | **(f) In sample mean $R^2$ (sd)** | | | | | |
| High | ***0.846*** | **0.841** | 0.553 | 0.547 | 0.536 | 0.525 | 0.759 | 0.773 | 0.755 |
| | (0.008) | (0.002) | (0.054) | (0.058) | (0.052) | (0.039) | (0.012) | (0.026) | (0.012) |
| Fair | ***0.765*** | **0.756** | 0.553 | 0.543 | 0.511 | 0.482 | 0.651 | 0.718 | 0.644 |
| | (0.014) | (0.004) | (0.065) | (0.070) | ( 0.064) | (0.040) | (0.018) | (0.024) | (0.019) |
| Low | ***0.522*** | 0.511 | 0.428 | 0.410 | 0.400 | 0.396 | 0.358 | **0.548** | 0.349 |
| | (0.027) | (0.018) | (0.041) | (0.030) | (0.018) | (0.007) | (0.025) | (0.019) | (0.025) |

**Web Table 8:** Simulation of 8 variables

a)Average number of true variables selected

| Senario | SNR | SuRF | Stability (0.6) | LASSO |
|---|---|---|---|---|
| | High | 2.95 (0.796) | 1.08 (0.273) | 2.11 (0.373) |
| S1 | Fair | 2.22 (0.645) | 1.11 (0.345) | 2.28 (0.697) |
| | Low | 1.99(0.438) | 1.10 (0.302) | 2.14 (0.725) |
| | High | 4.37 (1.390) | 1.23 (0.446) | 3.29 (0.518) |
| S2 | Fair | 3.08 (0.598) | 1.15 (0.386) | 2.96 (0.737) |
| | Low | 2.86 (0.551) | 0.99 (0.389) | 2.51 (0.689) |

b) Average number of noise variables selected

| | | | | |
|---|---|---|---|---|
| | High | 0.83 (0.792) | 5.46 (1.314) | 34.28 (14.600) |
| S1 | Fair | 0.42 (0.699) | 3.87 (1.353) | 19.33 (10.440) |
| | Low | 0.39 (0.618) | 2.89 (1.214) | 17.20 (8.837) |
| | High | 1.40 (0.791) | 2.86 (1.092) | 32.17 (12.254) |
| S2 | Fair | 0.53 (0.688) | 1.75 (0.845) | 24.18 (11.832) |
| | Low | 0.43 (0.607) | 1.25 (0.857) | 18.14 (11.889) |

c) Misclassification Error Rate

| | | | | |
|---|---|---|---|---|
| | High | 0.174 (0.028) | 0.235 (0.046) | 0.218 (0.035) |
| S1 | Fair | 0.246 (0.028) | 0.296 (0.039) | 0.274 (0.036) |
| | Low | 0.235 (0.023) | 0.311 (0.041) | 0.280 (0.036) |
| | High | 0.143 (0.030) | 0.255 (0.038) | 0.258 (0.051) |
| S2 | Fair | 0.239 (0.027) | 0.315 (0.028) | 0.317 (0.047) |
| | Low | 0.308 (0.027) | 0.369 (0.040) | 0.318 (0.037) |

**Web Table 9:** Frequency of selection for each variable over 100 simulations. The relative coefficients for each predictor are shown at the top of each scenario.

| Scenario | SNR | Method | A | A1 | A2 | B | B1 | B2 | C | D |
|---|---|---|---|---|---|---|---|---|---|---|
| | | | 1 | 1.5 | −0.5 | 1 | 2 | −0.5 | 1 | 1 |
| S1 | High | SURF | 79 | 57 | 17 | 0 | 100 | 0 | 0 | 42 |
| | | Stability (0.6) | 0 | 8 | 0 | 0 | 100 | 0 | 0 | 0 |
| | | LASSO | 1 | 97 | 1 | 0 | 100 | 0 | 0 | 12 |
| | Fair | SURF | 68 | 32 | 5 | 0 | 100 | 0 | 0 | 17 |
| | | Stability (0.6) | 8 | 1 | 0 | 0 | 100 | 0 | 0 | 2 |
| | | LASSO | 28 | 77 | 1 | 0 | 100 | 0 | 0 | 22 |
| | Low | SURF | 68 | 26 | 1 | 0 | 100 | 0 | 0 | 4 |
| | | Stability (0.6) | 7 | 3 | 0 | 0 | 100 | 0 | 0 | 0 |
| | | LASSO | 26 | 71 | 0 | 0 | 100 | 1 | 0 | 16 |
| | | | 1 | 1 | 2 | 1 | 1 | 2 | 2 | 1 |
| S2 | High | SURF | 14 | 100 | 100 | 100 | 1 | 38 | 46 | 38 |
| | | Stability (0.6) | 0 | 0 | 100 | 9 | 14 | 0 | 0 | 0 |
| | | LASSO | 0 | 0 | 100 | 88 | 46 | 93 | 0 | 2 |
| | Fair | SURF | 8 | 79 | 99 | 100 | 0 | 10 | 6 | 6 |
| | | Stability(0.6) | 0 | 0 | 99 | 7 | 9 | 0 | 0 | 0 |
| | | LASSO | 0 | 3 | 100 | 79 | 49 | 63 | 0 | 2 |
| | Low | SURF | 10 | 63 | 98 | 100 | 0 | 10 | 3 | 3 |
| | | Stability (0.6) | 0 | 0 | 89 | 1 | 9 | 0 | 0 | 0 |
| | | LASSO | 0 | 1 | 100 | 65 | 43 | 42 | 0 | 0 |

**Web Table 10:** Full results comparison among SuRF, Stability selection, VSURF, LASSO, Random Forest (RF) and SVM (Linear Kernel) for the pouchitis study and moving picture data

**a) Pouchitis study (Leave-one-out prediction mean test error (sd))**

| Site | SuRF | Stability Selection | VSURF | LASSO | RF | SVM |
|---|---|---|---|---|---|---|
| Pouch | 0.197 (0.047) | 0.197 (0.047) | 0.268 (0.053) | 0.282 (0.053) | 0.169 (0.044) | 0.211 (0.048) |
| Afferent limb | 0.254 (0.052) | 0.254 (0.052) | 0.254 (0.052) | 0.324 (0.056) | 0.225 (0.050) | 0.211 (0.048) |

**b) Moving picture**

| Site | SuRF | | Stability Selection | | | VSURF | | LASSO | | RF | SVM |
|---|---|---|---|---|---|---|---|---|---|---|---|
| | no. var | Test Error mean(sd) | Cut-off Probability | no. var | Test Error | no. var | Test Error mean(sd) | no. var | Test Error mean(sd) | Test Error mean(sd) | Test Error mean(sd) |
| Gut | *1* | 0.000 | 0.6 | *10* | 0.000 | *1* | 0.000 | *18* | 0.000 | 0.000 | 0.000 |
| | | | 0.7 | *10* | 0.006 (0.006) | | | | | | |
| | | | 0.8 | *6* | 0.000 | | | | | | |
| | | | 0.9 | *3* | 0.000 | | | | | | |
| Tongue | *3* | 0.053 (0.017) | 0.6 | *14* | 0.030 (0.013) | *3* | 0.018 (0.010) | *9* | 0.000 | 0.006 (0.006) | 0.024 (0.012) |
| | | | 0.7 | *13* | 0.053 (0.017) | | | | | | |
| | | | 0.8 | *10* | 0.018 (0.010) | | | | | | |
| | | | 0.9 | *8* | 0.000 | | | | | | |
| Left Palm | *2* | 0.024 (0.012) | 0.6 | *5* | 0.030 (0.013) | *3* | 0.061 (0.019) | *67* | 0.079 (0.021) | 0.079 (0.021) | 0.224 (0.032) |
| | | | 0.7 | *3* | 0.042 (0.016) | | | | | | |
| | | | 0.8 | *3* | 0.042 (0.016) | | | | | | |
| | | | 0.9 | *2* | 0.030 (0.013) | | | | | | |
| Right Palm | *2* | 0.025 (0.012) | 0.6 | *7* | 0.080 (0.021) | *4* | 0.025 (0.012) | *45* | 0.129 (0.026) | 0.037 (0.015) | 0.288 (0.035) |
| | | | 0.7 | *3* *3* | 0.061 (0.019) | | | | | | |
| | | | 0.8 | *3* | 0.061 (0.019) | | | | | | |
| | | | 0.9 | *2* | 0.067 (0.020) | | | | | | |
| Left palm predicts right palm | | 0.020 (0.006) | 0.6 | | 0.034 (0.008) | | 0.014 (0.005) | | 0.049 (0.010) | 0.152 (0.016) | 0.148 (0.016) |
| | | | 0.7 | | 0.028 (0.007) | | | | | | |
| | | | 0.8 | | 0.028 (0.007) | | | | | | |
| | | | 0.9 | | 0.020 (0.006) | | | | | | |

**Web Table 11:** Simulation results for changing the proprotion of subsampling in Study 2 (fair SNR senario for the binary case)

| proportion | Frequency of no. of true variables selected | | | Average no. of noise variables (sd) | Mean misclassification error (sd) |
|---|---|---|---|---|---|
| | **3** | **2** | **1** | | |
| 50% | 80 | 19 | 1 | 0.77 (0.920) | 0.191 (0.029) |
| 60% | 81 | 18 | 1 | 0.72 (0.889) | 0.191 (0.030) |
| 70% | 81 | 18 | 1 | 0.74 (0.883) | 0.191 (0.029) |
| 80% | 82 | 17 | 1 | 0.71 (0.913) | 0.191 (0.028) |
| 90% | 82 | 18 | 0 | 0.69 (0.895) | 0.191 (0.028) |

**Web Table 12:** Testing the $p$-values

| | Scenario | SNR | all true selected | noise variables | $p$-value | significant |
|---|---|---|---|---|---|---|
| Simulation 1 | S1 | High | 100 | 2 | 0.020 | 0.964 |
| | | Fair | 98 | 6 | 0.058 | 0.411 |
| | | Low | 95 | 3 | 0.031 | 0.869 |
| | S2 | High | 100 | 6 | 0.057 | 0.429 |
| | | Fair | 100 | 11 | 0.099 | 0.022 |
| | | Low | 97 | 4 | 0.040 | 0.742 |
| | S3 | High | 100 | 5 | 0.048 | 0.599 |
| | | Fair | 66 | 2 | 0.029 | 0.854 |
| | | Low | 35 | 0 | 0 | 1.000 |
| | S4 | High | 19 | 1 | 0.05 | 0.623 |
| | | Fair | 9 | 1 | 0.1 | 0.370 |
| | | Low | 8 | 0 | 0 | 1.000 |
| Simulation 2 | Binary response | High | 71 | 1 | 0.014 | 0.974 |
| | | Fair | 82 | 3 | 0.035 | 0.797 |
| | | Low | 99 | 3 | 0.029 | 0.886 |
| | Continuous response | High | 99 | 1 | 0.01 | 0.994 |
| | | Fair | 97 | 6 | 0.058 | 0.402 |
| | | Low | 80 | 4 | 0.048 | 0.601 |

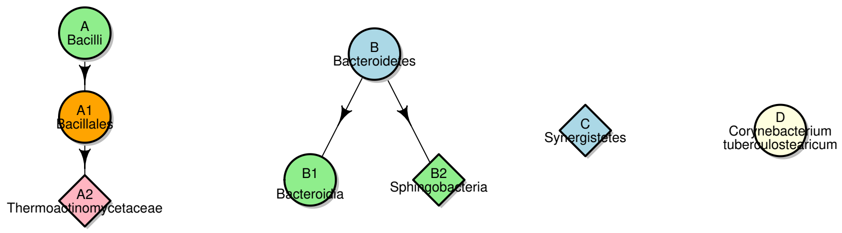


**Web Figure 1:** Variables used in the simulation. Circles represent abundant taxa, while diamonds represent rare taxa. Colours represent taxonomic level: blue — phylum; green — class; orange — order; pink — family; light yellow — species

**Web Figure 2:** Permutation distributions of Likelihood Ratio (LR) in training samples from real data sets.

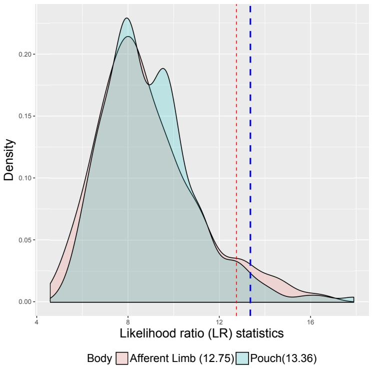


**(a)** Pouch and Afferent Limb

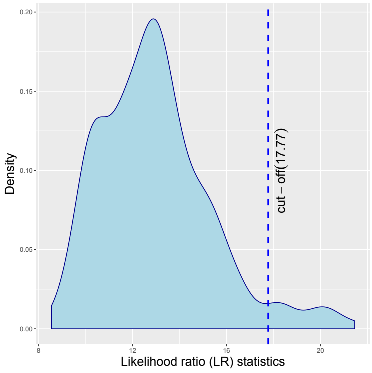


**(b)** Gut

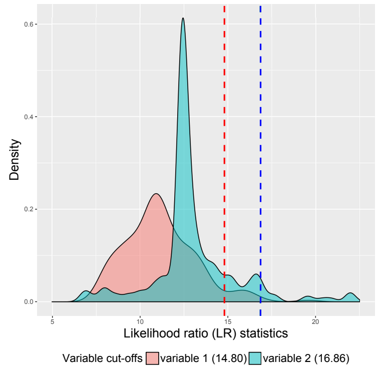


**(c)** Tongue: variables 1 and 2

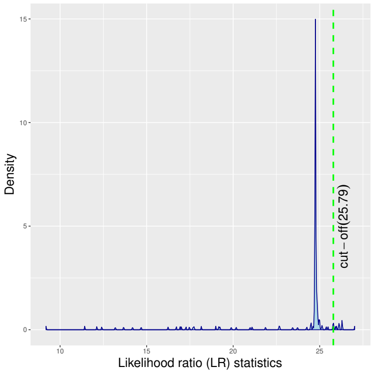


**(d)** Tongue: third variable

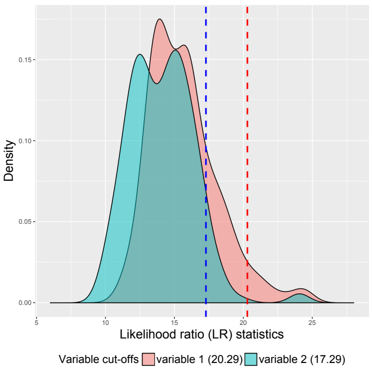


**(e)** Left palm

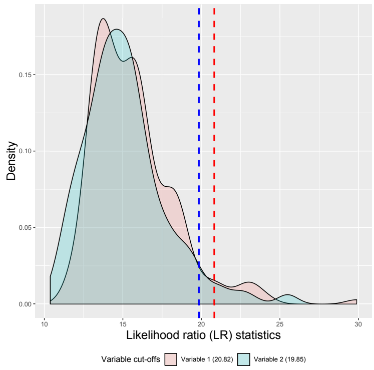


**(f)** Right palm

**Web Figure 3:** ROC curve for Bacteroidetes as a predictor of inflammation

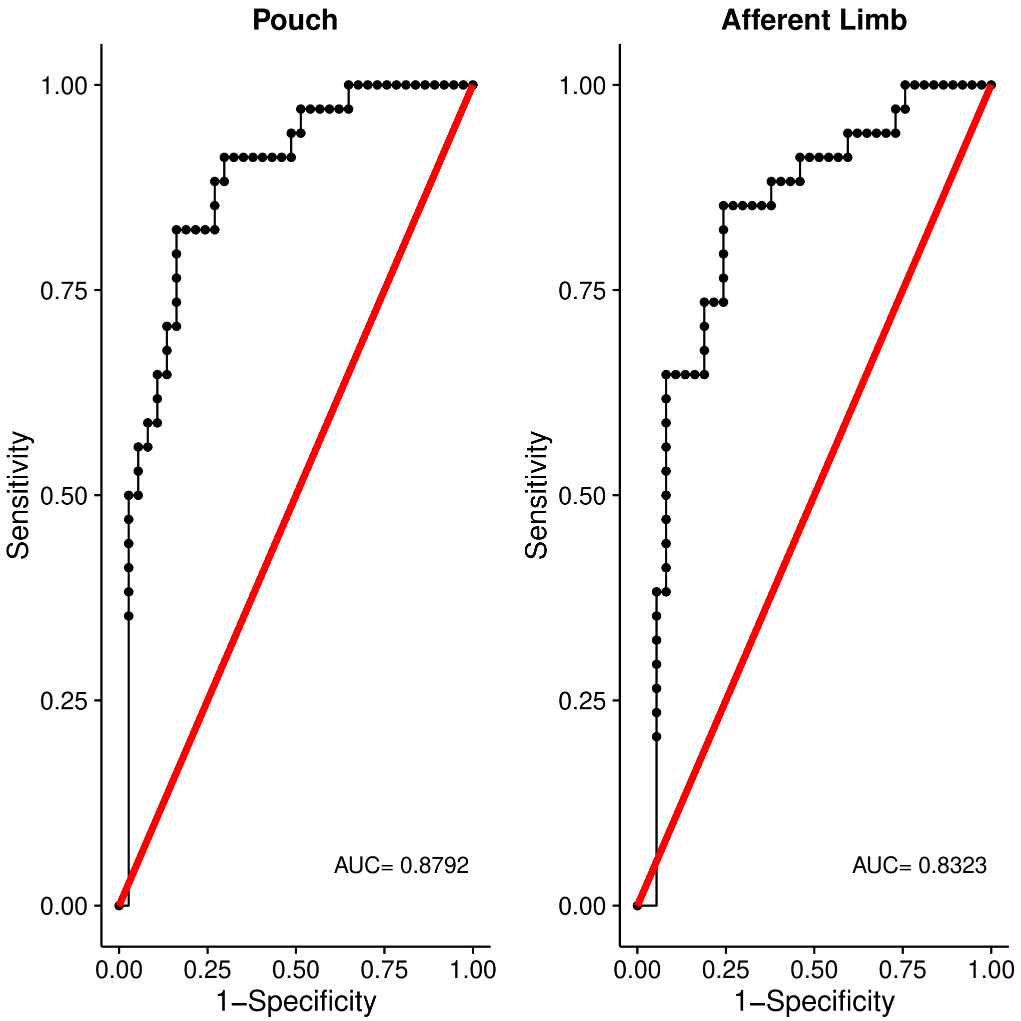

**Web Figure 4:** Prediction of test samples from gut, tongue, left and right palm

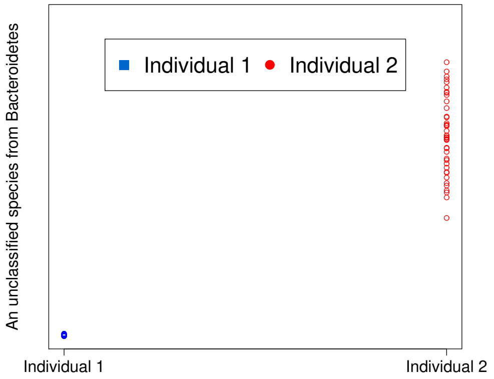


**(a)** Gut

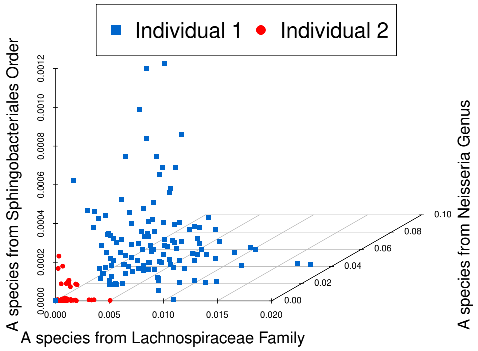


**(b)** Tongue

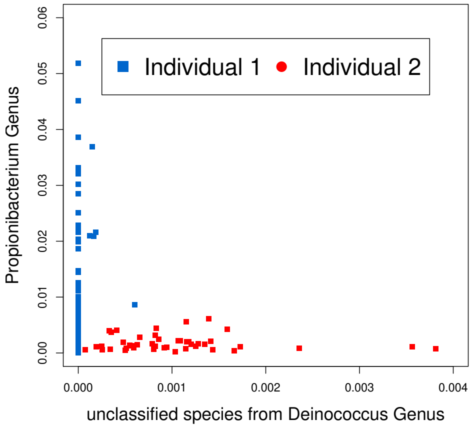


**(c)** Left palm

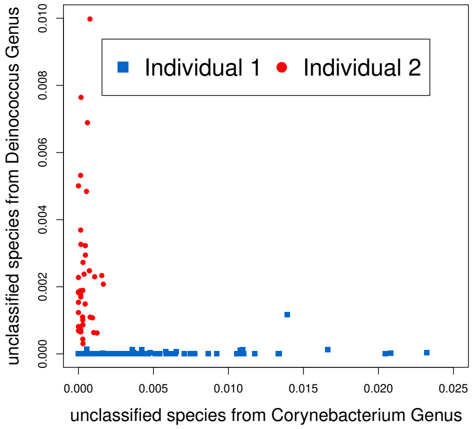


**(d)** Right palm
